# Supplementary material for: Island dynamics and anisotropy during vapor phase epitaxy of m-plane GaN
Source: arXiv:1706.09955 ancillary file (2017-06-29)
Supplement: Supplementary file 1 [file 2017_Perret_Supplemental_v1.pdf]

# Supplemental Material for "Island dynamics and anisotropy during vapor phase epitaxy of m-plane GaN"

Edith Perret,[1,2] Dongwei Xu,[1] M. J. Highland,[1] G. B. Stephenson,[1] P. Zapol,[1] P. H. Fuoss,[1,a)] A. Munkholm,[3] and Carol Thompson[4,b)]

[1)] *Materials Science Division, Argonne National Laboratory, Argonne, IL 60439 USA*
[2)] *University of Fribourg, Department of Physics and Fribourg Center for Nanomaterials, Chemin du musée 3, CH-1700 Fribourg, Switzerland*
[3)] *Munkholm Consulting, Mountain View, CA 94043 USA*
[4)] *Department of Physics, Northern Illinois University, DeKalb IL 60115 USA*

(Dated: 30 June 2017)

This supplemental material contains a description of experimental conditions and methods, methods of fitting the data to obtain island spacings $S_z$ and $S_y$, and a comparison of the island spacings $S_z$ to the step-flow boundary obtained from CTR intensity oscillations.

## I. EXPERIMENTAL CONDITIONS AND METHODS

Methods were substantially the same as described previously.[1] Grazing-incidence x-ray surface scattering measurements[2] were performed at undulator beamline 12ID-D of the Advanced Photon Source in a vertical flow MOVPE chamber mounted on a z-axis surface diffractometer.[3,4] An x-ray energy of 28.26 keV was used to penetrate the 2-mm-thick quartz walls of the chamber. The grazing angle was set to the critical angle, $\alpha = 0.09°$, to obtain maximum surface sensitivity. Diffracted x-rays were observed with a pixel array detector.[5]

The single-crystal GaN substrate, crystal "C" of the previous work,[1] was purchased from a commercial supplier.[6] The angle of the surface with respect to the $(1\,0\,\bar{1}\,0)$ planes, determined by atomic force microscopy, was 0.4°, giving terraces of width $W = 400$ Å between $(1\,0\,\bar{1}\,0)$ steps, at an azimuth of 10° from $[0\,0\,0\,\bar{1}]$. To prepare a clean surface before the growth mode studies, crystals were etched in a 10% HCl solution for 5 min and a 400-Å-thick buffer layer of GaN was grown *in situ* at 1250 K.

Triethylgallium (TEGa) and ammonia ($NH_3$) were used as precursors and nitrogen as carrier gas. The total chamber pressure was 267 mbar, and the total reactive gas flow was 4.7 slpm. The sample temperature was calibrated to within ±5 K for the relevant gas flow conditions using optical interferometry measurements of the thermal expansion of a standard sapphire substrate.[7] For these growth studies, the $NH_3$ flow was kept constant at 2.7 slpm, and the TEGa flow was used to control growth. (The $NH_3$ flow used, $1.2 \times 10^5 \mu$mol/min, represents a large oversupply, with a V/III ratio $> 10^5$. We observed that the growth behavior is typically independent of $NH_3$ flow from 2.7 down to 0.01 slpm.) Growth rates were determined by the x-ray oscillation period under layer-by-layer conditions,[1] and by *in situ* optical interferometry measurements of film thickness under step-flow conditions.[3] Over the complete range of conditions studied, we found that the growth rate was independent of temperature and proportional to the TEGa supply rate, with a growth rate of $1.0 \pm 0.1$Å/s for each $\mu$mol/min of TEGa supplied. This indicates that the growth rate is limited by precursor transport rather than surface kinetics.[8] Extrapolation to zero TEGa supply gives a zero growth rate, which indicates that there is negligible GaN re-evaporation under the conditions studied.

## II. METHOD OF FITTING TO GET $\Delta L_{pk}$ AND $S_z$

The sequence of images obtained from the area detector during each growth run were first plotted in reciprocal space coordinates. The reciprocal lattice units used were relative to room-temperature GaN, $a_0 = 3.19$ Å, $c_0 = 5.18$ Å. Values of $H$, $K$, and $L$ reciprocal space coordinates were obtained for every detector pixel using the orientation matrix determined for the sample, the spectrometer angles, and the relative angles of each pixel of the area detector with respect to its reference pixel.[9] Because the CTR and the diffuse scattering from the islands are extended in the surface normal $H$ direction, the images were projected onto the $KL$ plane to analyze the in-plane diffuse scattering from the islands. Figures S.1 and S.2 show typical images before growth and after 0.5 ML of growth, respectively, plotted in the $KL$ plane.

One can see from Fig. S.1 before growth that the resolution function obtained for the CTR using the grazing-incidence geometry is asymmetric in the $KL$ plane, tilted in a direction corresponding to $dL/dK \approx 5$. Figure S.2 after 0.5 ML of growth is plotted using $\Delta K$ and $\Delta L$ relative to the peak position before growth. The central CTR intensity at $\Delta K = \Delta L = 0$ is minimum and satellite peaks appear at positions $\pm\Delta L_{pk}$ around the CTR. Each of these peaks is convolved with the same tilted resolution function. To obtain the diffuse scattering profiles $I(L,t)$ in the $L$ direction shown in Fig. 3 of the main paper, for each point we integrated the signal within each

[a)] current address: SLAC National Accelerator Laboratory, Menlo Park, CA 94025 USA
[b)] correspondence to: cthompson@niu.edu

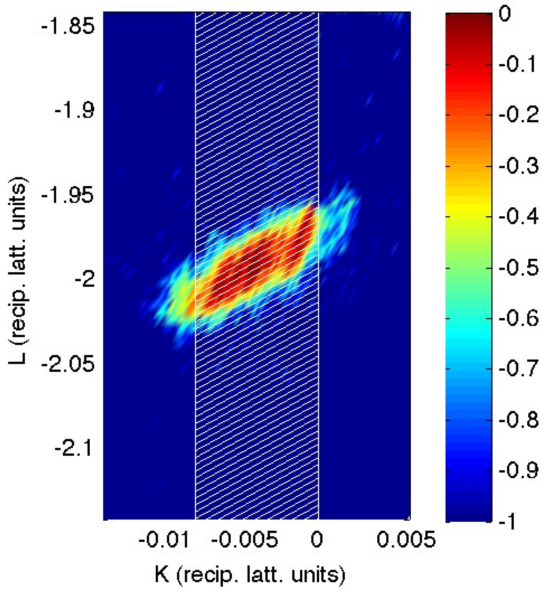


FIG. S.1. Typical diffuse intensity distribution in the $KL$ plane around the $(H\,0\,\overline{H}\,\overline{2})$ CTR near $H = 0.5$ prior to growth, showing the CTR with no diffuse scattering. Colorbar gives $\log_{10}(I)$. Also shown (white outlines) are the regions used to integrate the intensity to produce a profile as a function of $L$ only.

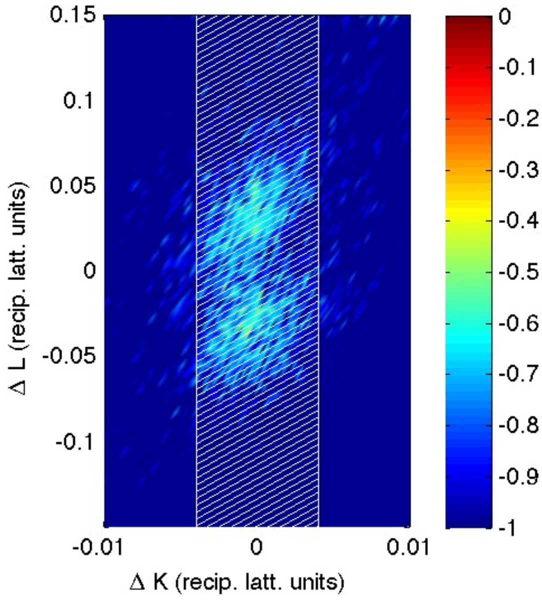


FIG. S.2. Typical diffuse intensity distribution in the $KL$ plane around the $(H\,0\,\overline{H}\,\overline{2})$ CTR near $H = 0.5$ after growth of 0.5 ML, showing the satellite diffuse scattering peaks from the islands. Colorbar gives $\log_{10}(I)$. Also shown (white outlines) are the regions used to integrate the intensity to produce a profile as a function of $L$ only.

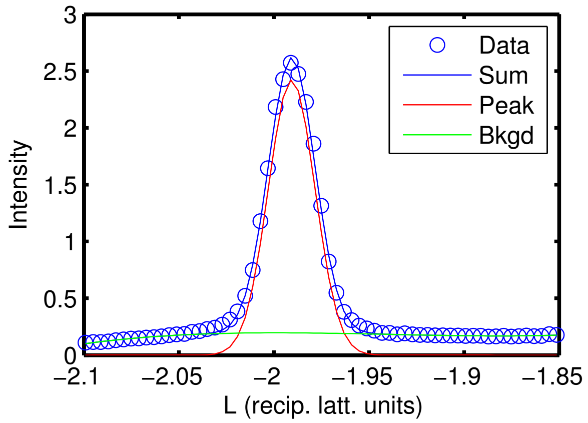


FIG. S.3. Typical diffuse intensity distributions around the CTR in the $L$ direction prior to growth, showing the CTR with no diffuse scattering. Also shown are fits to extract the peak position, shape, and background.

of the white parallelograms shown in Figs. S.1 and S.2, which were aligned with the resolution function to preserve highest resolution in $L$. We used integration regions of width 0.008 r.l.u. in $L$ over a range $\Delta K = \pm 0.004$. A typical sequence of these profiles as a function of time during growth is shown in Fig. 2 of the main paper.

The peak position $\Delta L_{pk}$ at 0.5 ML coverage was extracted for each growth run by fitting the profile for times near the first minimum in the CTR intensity. The first step in this process was to fit the profile prior to growth to obtain the background and the position and width of the initial CTR. The background was obtained by fitting a cubic polynomial to the tails on each side of the central peak. A Gaussian peak shape was found to fit well the background-subtracted CTR, as shown in Fig. S.3. The initial peak position, used to set the zero of $\Delta K$ and $\Delta L$, is slightly displaced from integer values. This accounts for the temperature dependence of the lattice parameters, and any small misalignments of the crystal orientation matrix arising from temperature cycling. The background obtained from the pre-growth scattering was subtracted from all profiles in the time sequence. The remaining signal profile at the time corresponding to 0.5 ML was fit using a pair of identical Lorentzians displaced equally on opposite sides of the initial CTR position, as well as a central Gaussian peak with the same position and width as the initial CTR peak. The double Lorentzian shape was found to work well for the diffuse scattering; it overestimates the tails, but fits well near the peak where it matters. To reduce the number of fit parameters, the width of the Lorentzians was forced to be proportional to their displacement, with a fixed ratio of 1.75 set by the average of the (reasonably constant) ratios obtained from unforced fits to the 15 datasets that have most well-defined satellite peaks. This kept the peak displacement consistently determined within the width of the overall scattering for the datasets without well-

defined satellite peaks. The final fits thus had three free parameters: the diffuse (Lorentzian) position $\Delta L_{pk}$, and the intensities of the diffuse and central peak (CTR) components. The CTR component was needed because some of the datasets have a residual central peak, depending upon how well our time sequence captured the exact 0.5 ML condition. Typical fits are shown in Fig. 3 of the main paper.

Datasets corresponding to conditions in the step-flow growth mode (higher $T$ and lower $G$) did not show significant diffuse intensity from islands. We excluded these data sets from the analysis of island spacing as a function of $T$ and $G$ using a criterion based on the normalized CTR oscillation amplitude $\Delta I \equiv (I_1 - I_{0.5})/I_0$, where $I_0$, $I_{0.5}$, and $I_1$ are the CTR intensities at 0, 0.5, and 1 ML of growth. The growth mode map based on $\Delta I$ from these datasets was shown in our previous publication.[1] We found that accurate satellite peak positions $\Delta L_{pk}$ were obtained for all the conditions giving $\Delta I > 0.11$, indicating a layer-by-layer growth mode. The peak positions for these 26 conditions were used to obtain the values of $S_z = c_0/\Delta L_{pk}$ shown in Fig. 4(a) in the main paper.

While Fig. 4 in the main paper displays certain groups of $S_z$ values as being at the same temperature $T$ or the same growth rate $G$, there was some variation in the measured $T$ or $G$ values within each group. The $T$ values were the same within ±1 K, while the $G$ values were the same within ±10%. The fit of Eq. (1) to the 26 values of $S_z$ used the measured values of $T$ and $G$ for each condition. The fit curves shown with each group of values in Fig. 4 were calculated using the average $T$ or average $G$ for that group.

## III. METHOD OF FITTING TO GET $\Delta K_{pk}$ AND $S_y$

We analyzed small changes in the peak width to estimate the island spacing in the $[1\,\overline{2}\,1\,0]$ direction. We first obtained the intensity distribution in the $K$ direction, $I(K,t)$, in a manner similar to that described above for $I(L,t)$. However, the tilt of the resolution function in the $KL$ plane was disregarded in determining $I(K,t)$. Using the same starting intensity distributions as a function of $K$ and $L$ derived above, we simply integrated the distributions in the $L$ direction, as shown in Figs. S.4 and S.5. We used integration regions of width 0.0008 in $K$, over a range $\Delta L = \pm 0.14$ r.l.u. centered about the peak position determined from the pre-growth scattering.

We determined the peak widths in the $K$ direction from these distributions, both from the pre-growth scattering and from the scattering at 0.5 ML of growth. First we fit and subtracted the background as above for the analysis of the $I(L,t)$. We found that the integral full width $IFW_K$, defined as the integrated intensity divided by the peak intensity (both above background), was the width statistic most sensitive to small changes. To obtain $IFW_K$, the peak intensity was determined by averaging

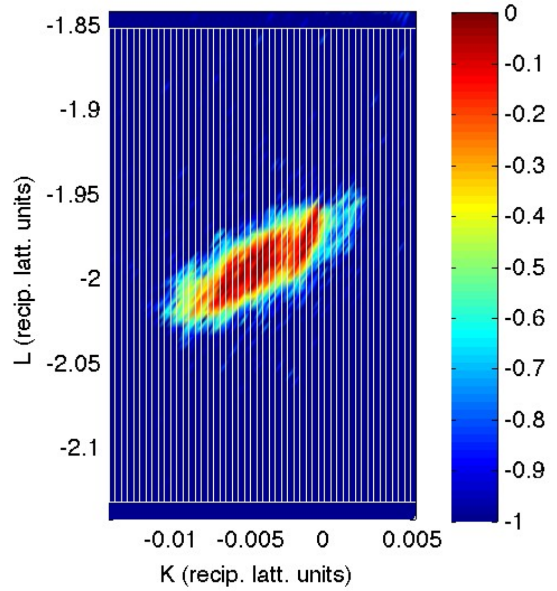


FIG. S.4. Typical diffuse intensity distribution in the $KL$ plane around the $(H\,0\,\overline{H}\,\overline{2})$ CTR near $H = 0.5$ prior to growth, showing the CTR with no diffuse scattering. Colorbar gives $\log_{10}(I)$. Also shown (white outlines) are the regions used to integrate the intensity to produce a profile as a function of $K$ only.

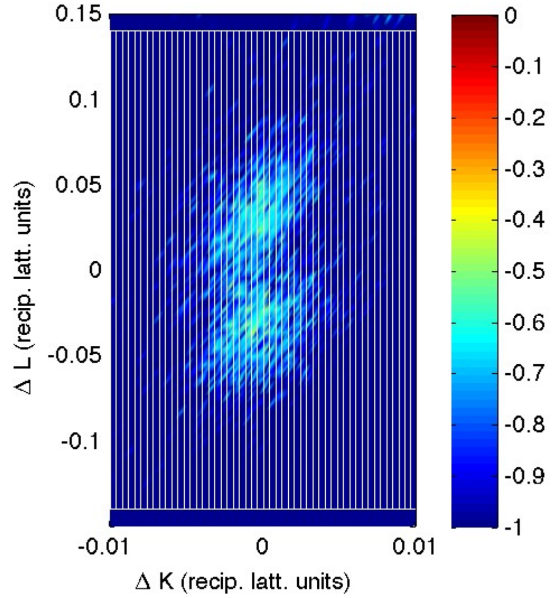


FIG. S.5. Typical diffuse intensity distribution in the $KL$ plane around the $(H\,0\,\overline{H}\,\overline{2})$ CTR near $H = 0.5$ after growth of 0.5 ML, showing the satellite diffuse scattering peaks from the islands. Colorbar gives $\log_{10}(I)$. Also shown (white outlines) are the regions used to integrate the intensity to produce a profile as a function of $K$ only.

the intensity over a range of $\Delta K = \pm 0.0015$ r.l.u.

All datasets with island spacings $S_z > 15$ nm showed increases in the peak width at 0.5 ML of growth $IFW_K(0.5ML)$ relative to the pre-growth width $IFW_K(0ML)$. We estimated the contribution to the peak width from islands at 0.5 ML of growth using the formula

$$\Delta IFW_K = (IFW_K(0.5ML)^2 - IFW_K(0ML)^2)^{1/2}. \quad \text{(S.1)}$$

This change in peak width can be attributed to the summation of two peaks displaced by amounts $\pm\Delta K_{pk}$ due to islands, as in the analysis of $I(L,t)$. However, in this case, the displacement is small relative to the resolved peak width, and we see a broadened single peak rather than two resolved peaks. In this limit, the displacement can be related to the change in peak width by $\Delta K_{pk} \approx 0.4\Delta IFW_K$. The island spacing in the $[1\,\bar{2}\,1\,0]$ direction can be obtained from the displacement in the $K$ direction by $S_y = a_0/\Delta K_{pk}$.

Errors in estimates of $S_y$ obtained from small changes in peak widths are relatively large, likely larger than the spread in the data points of Fig. 5 of the main paper because of potential systematic errors. Nevertheless the trend in the estimates indicates higher island anisotropy at lower growth rates.

## IV. COMPARISON OF ISLAND SPACING AND STEP-FLOW BOUNDARY

In our previous study,[1] the boundary between step-flow and layer-by-layer growth modes was determined by analysis of the amplitude $\Delta I$ of the oscillations in the CTR intensity. We can quantitatively compare that growth mode boundary with the dependence of $S_z$ on $G$ and $T$ observed here to test the hypothesis of whether the boundary corresponds to an average island spacing at 0.5 ML equal to the average terrace width, $S_z = W$. The boundary previously determined from $\Delta I$ for $W =$ 400 Å was[1]

$$G_{SF} = A_{SF}\exp(-E_{SF}/kT) \quad \text{(S.2)}$$

with $E_{SF} = 2.8 \pm 0.3$ eV and $\log_{10}[A_{SF}(\text{Å/s})] = 13.5 \pm 1.4$. The boundary calculated from the island spacing fit is $E_{SF} = E_S = 2.70 \pm 0.18$ eV and $\log_{10}[A_{SF}(\text{Å/s})] = \log_{10}[G_S(\text{Å/s})] - (1/n)\log_{10}(W/a_0) = 12.7 \pm 1.0$. These are in good agreement, supporting the hypothesis.

## ACKNOWLEDGMENTS

Work supported by the U.S. Department of Energy (DOE), Office of Science, Office of Basic Energy Sciences, Division of Materials Sciences. Use of beamline 12ID-D of the Advanced Photon Source, a DOE Office of Science User Facility operated for the Office of Science by Argonne National Laboratory, was supported under contract DE-AC02-06CH11357.

[1] E. Perret, M. J. Highland, G. B. Stephenson, S. K. Streiffer, P. Zapol, P. H. Fuoss, A. Munkholm, and C. Thompson, "Real-time x-ray studies of crystal growth modes during metal-organic vapor phase epitaxy of GaN on c- and m-plane single crystals," Applied Physics Letters **105**, 051602 (2014).

[2] I. K. Robinson and D. J. Tweet, "Surface x-ray diffraction," Reports on Progress in Physics **55**, 599–651 (1992).

[3] G. B. Stephenson, J. A. Eastman, O. Auciello, A. Munkholm, C. Thompson, P. H. Fuoss, P. Fini, S. P. DenBaars, and J. S. Speck, "Real-time x-ray scattering studies of surface structure during metalorganic chemical vapor deposition of GaN," MRS Bulletin **24**, 21 (1999).

[4] A. Munkholm, G. B. Stephenson, J. A. Eastman, O. Auciello, M. V. R. Murty, C. Thompson, P. Fini, J. S. Speck, and S. P. DenBaars, "In situ studies of the effect of silicon on GaN growth modes," Journal of Crystal Growth **221**, 98–105 (2000), proc Tenth Int Conf Metalorganic Vapor Phase Epitaxy.

[5] P. Kraft, A. Bergamaschi, C. Broennimann, R. Dinapoli, E. F. Eikenberry, B. Henrich, I. Johnson, A. Mozzanica, C. M. Schlepütz, P. R. Willmott, and B. Schmitt, "Performance of single-photon-counting PILATUS detector modules," Journal of Synchrotron Radiation **16**, 368–375 (2009).

[6] Kyma Technologies, 8829 Midway West Rd Raleigh, NC 27612, USA, http://www.kymatech.com.

[7] G. Ju, M. J. Highland, A. Yanguas-Gil, C. Thompson, J. A. Eastman, H. Zhou, S. M. Brennan, G. B. Stephenson, and P. H. Fuoss, "An instrument for in situ coherent x-ray studies of metal-organic vapor phase epitaxy of III-nitrides," Review of Scientific Instruments **88**, 035113 (2017).

[8] G. B. Stringfellow, "Fundamentals of vapor phase epitaxial growth processes," AIP Conference Proceedings **916**, 48–68 (2007).

[9] M. Lohmeier and E. Vlieg, "Angle calculations for a six-circle surface x-ray diffractometer," Journal of Applied Crystallography **26**, 706–716 (1993).
